# Supplementary material for: Interactive Gibson Benchmark (iGibson 0.5): A Benchmark for Interactive Navigation in Cluttered Environments
Source: arXiv:1910.14442 source file (2021-08-09)
Supplement: Supplementary file 1 [file appendix.tex]

\appendix

\color{blue}
\subsection{Additional Experimental Results}
In this section, we provide additional experimental results that could give us some insights about how different interactive navigation models perform on different robotics platforms. 

Fig.~\ref{fig:robot_platform_comp} compares the interactive navigation metrics between Turtlebot and Fetch robot. As can be seen from the scatter plot, Fetch is able to achieve the same path efficiency with higher effort efficiency. This is because Fetch is a much heavier robot than Turtlebot, and the effort efficiency takes into account the weight of the robot. Heavier robot is able to achieve higher effort efficiency as the objects moved are much lighter than the robot itself. 

\begin{figure}[h]
  \begin{center}
    \includegraphics[width=0.96\columnwidth]{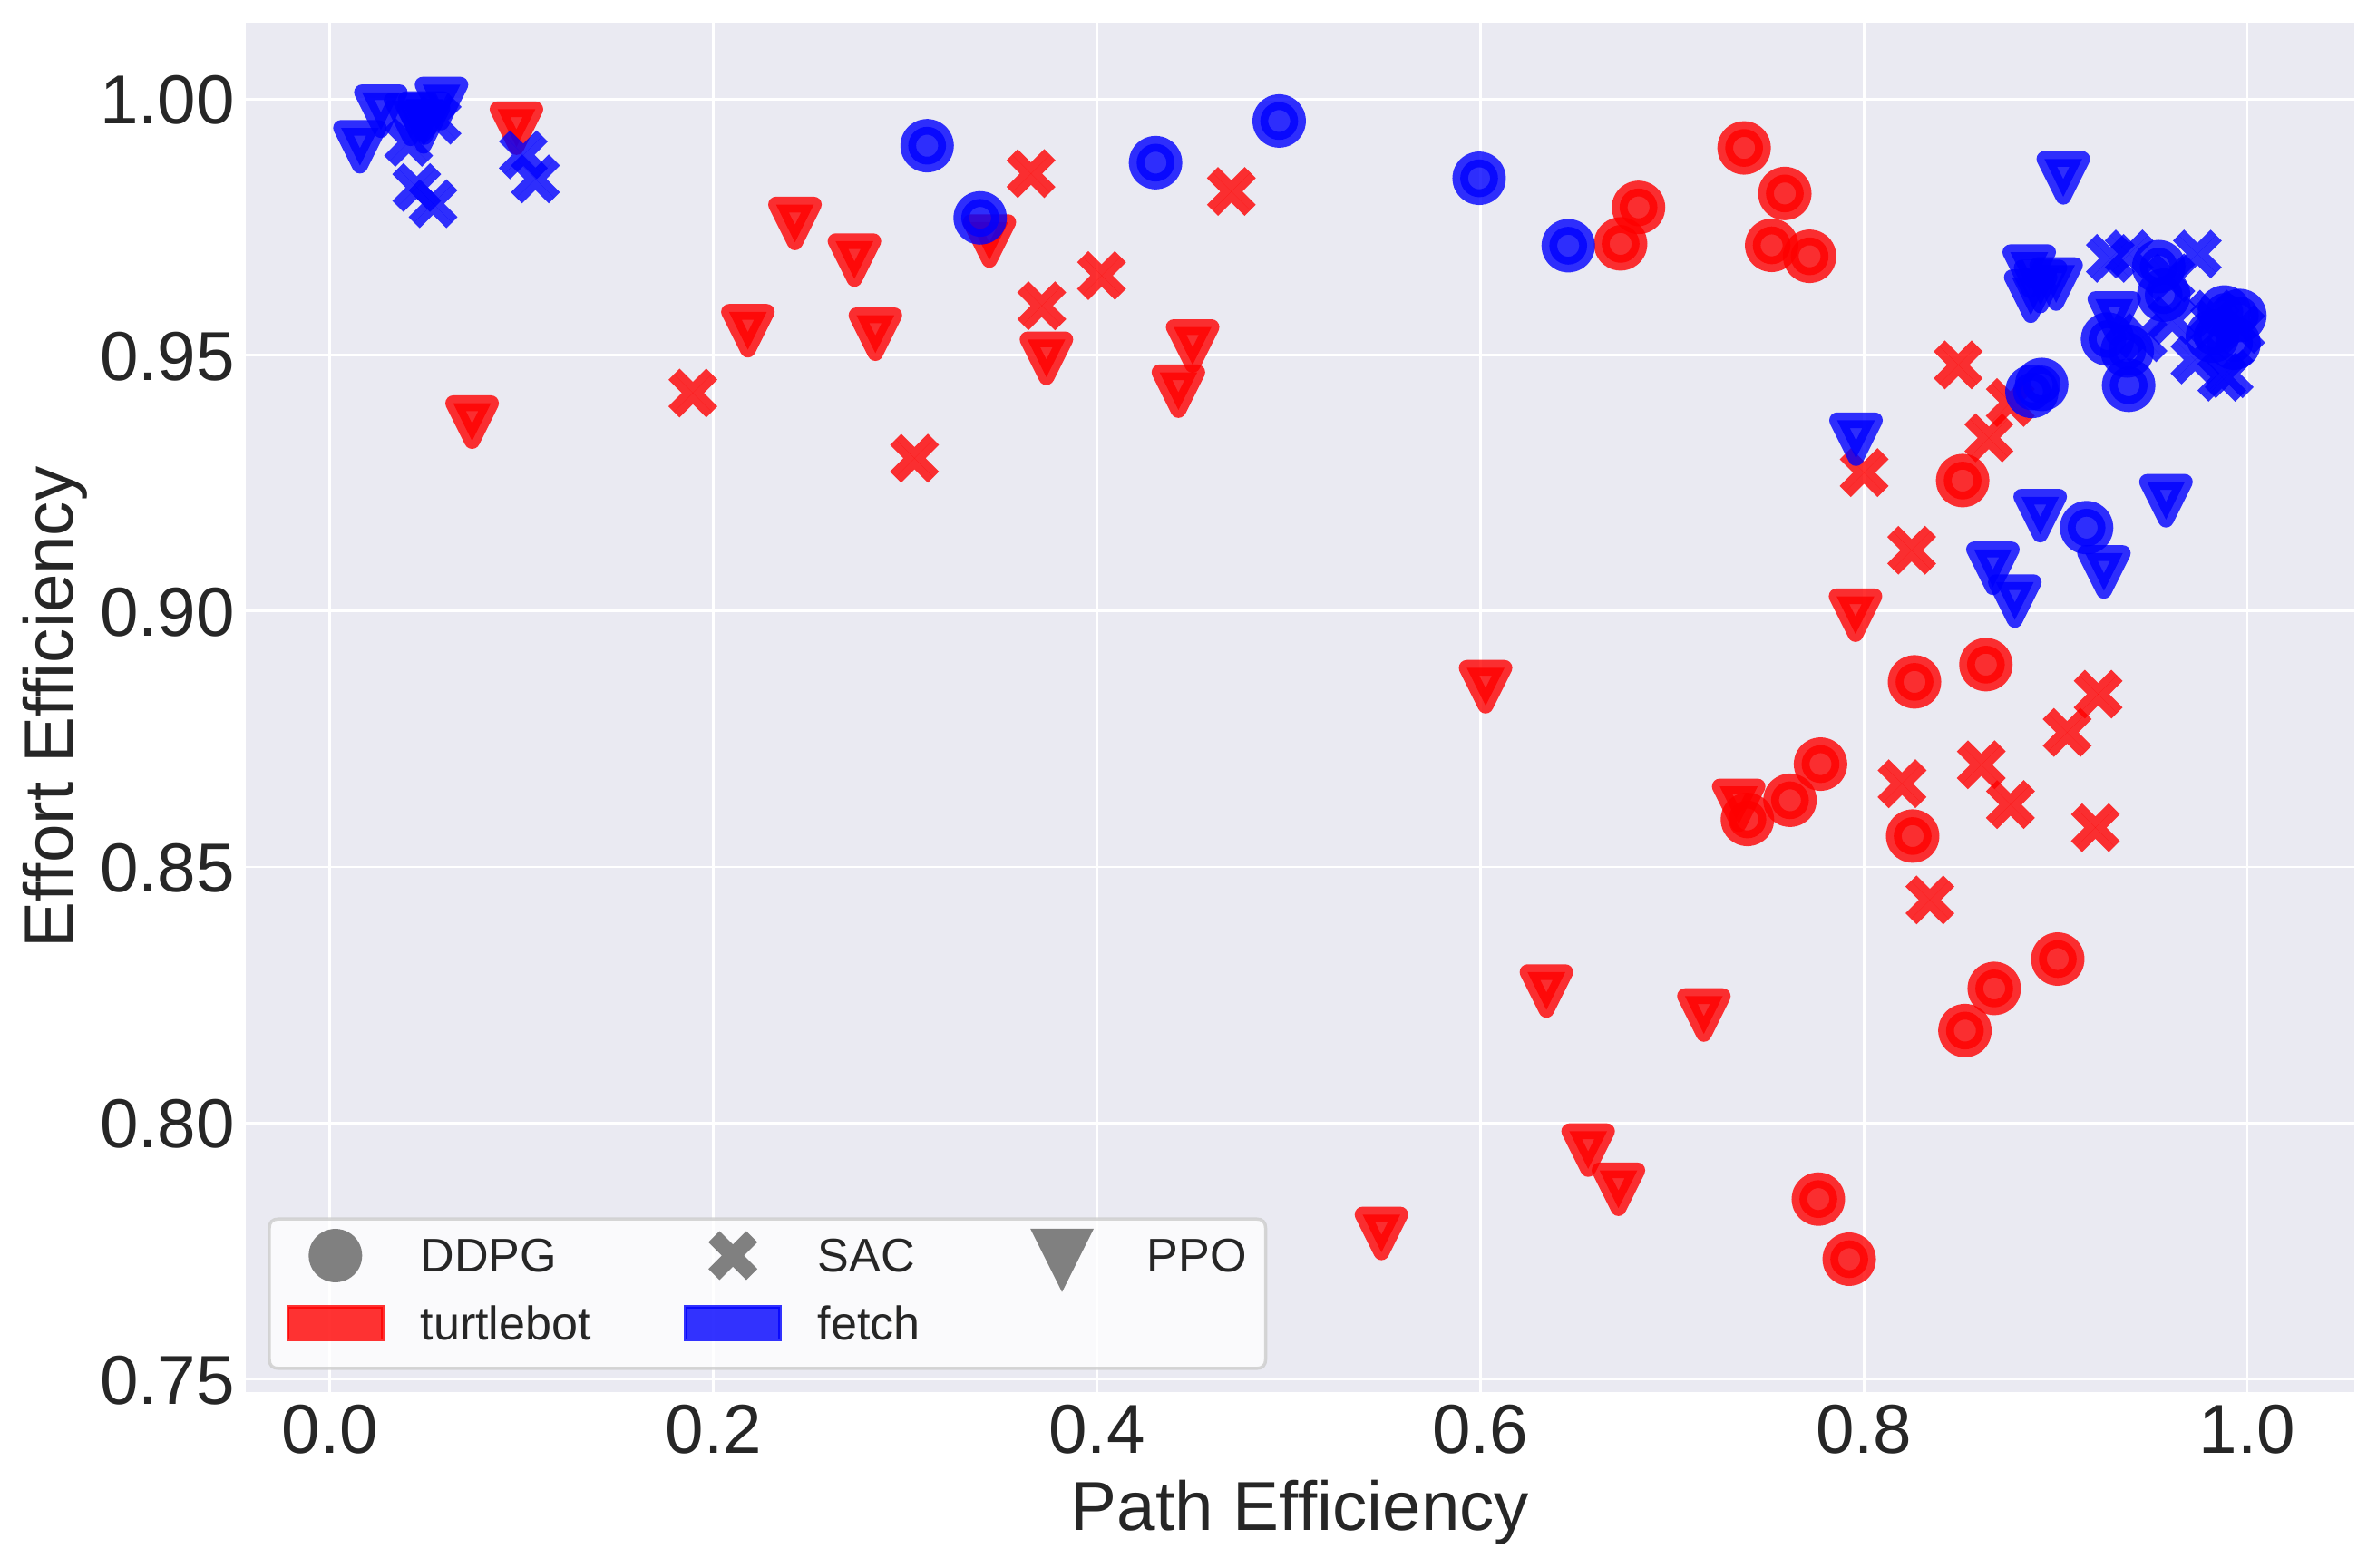}
  \end{center}
  	\caption{Comparison of Turtlebot and Fetch. Because Fetch carries more weight, it is able to achieve success navigation with higher effort efficiency.}
	\label{fig:robot_platform_comp}
\end{figure}

Fig.~\ref{fig:dd_kd} shows that the two terms in effort efficiency are highly correlated. This is just a sanity check that each term of the effort efficiency makes sense. 

\begin{figure}[h]
  \begin{center}
    \includegraphics[width=0.96\columnwidth]{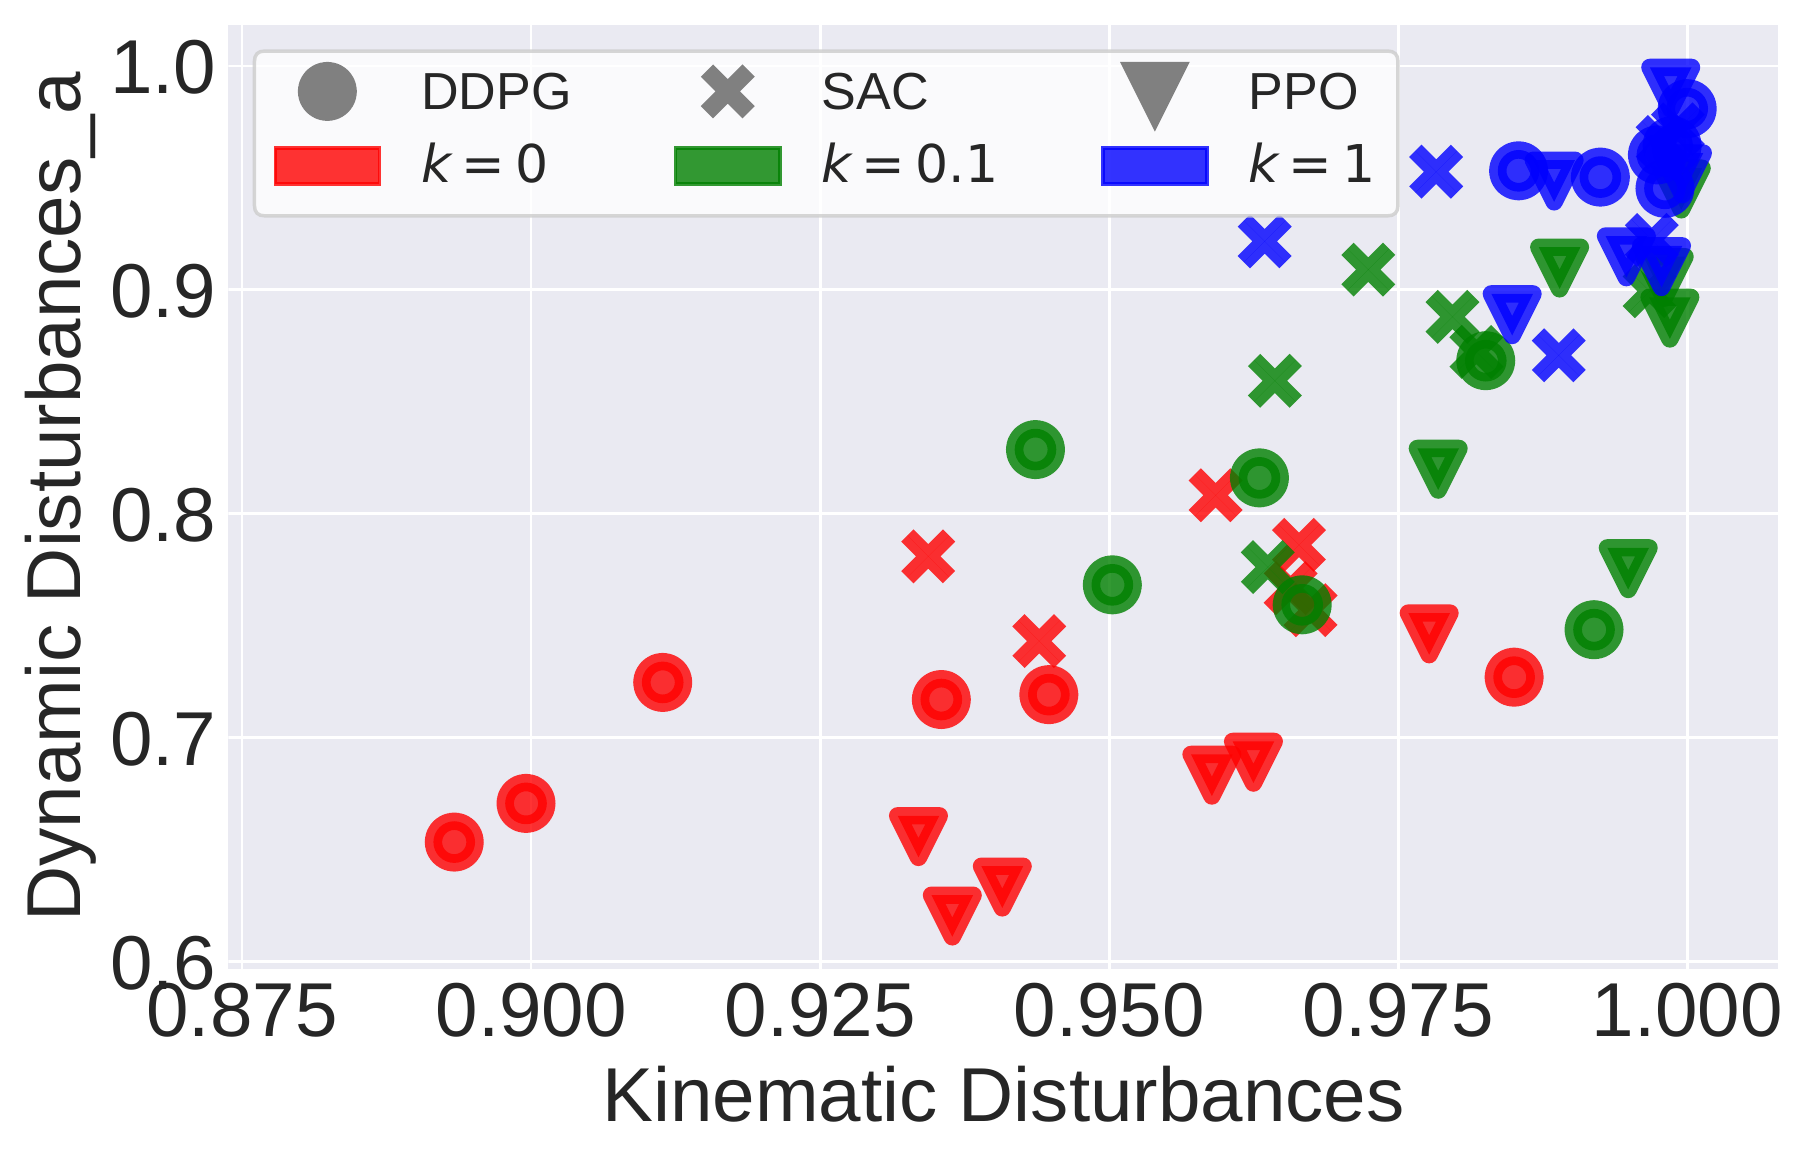}
  \end{center}
  	\caption{Dynamic disturbances and Kinematic disturbances are  correlated.}
	\label{fig:dd_kd}
	\vspace{-4mm}
\end{figure}

%\begin{figure}[t]
%  \begin{center}
%    \includegraphics[width=0.97\columnwidth]{figures/t%wo_type_of_dynamic_disturbance.pdf}
%  \end{center}
%  	\caption{Two types of dynamic disturbances are highly correlated.}
%	\label{fig:examples}
%\end{figure}

In the main text, we showed the trade-off between path and efficiency for Fetch so here we included the trade-off plot for Turtlebot in Fig.~\ref{fig:trade_off_turtlebot}. The results are overall similar. In the main text we showed the interactive navigation score at different $\alpha$ for Turtlebot so we include interactive navigation score for Fetch in Fig.~\ref{fig:ins_fetch}. 

\begin{figure}[h]
  \begin{center}
    \includegraphics[width=0.96\columnwidth]{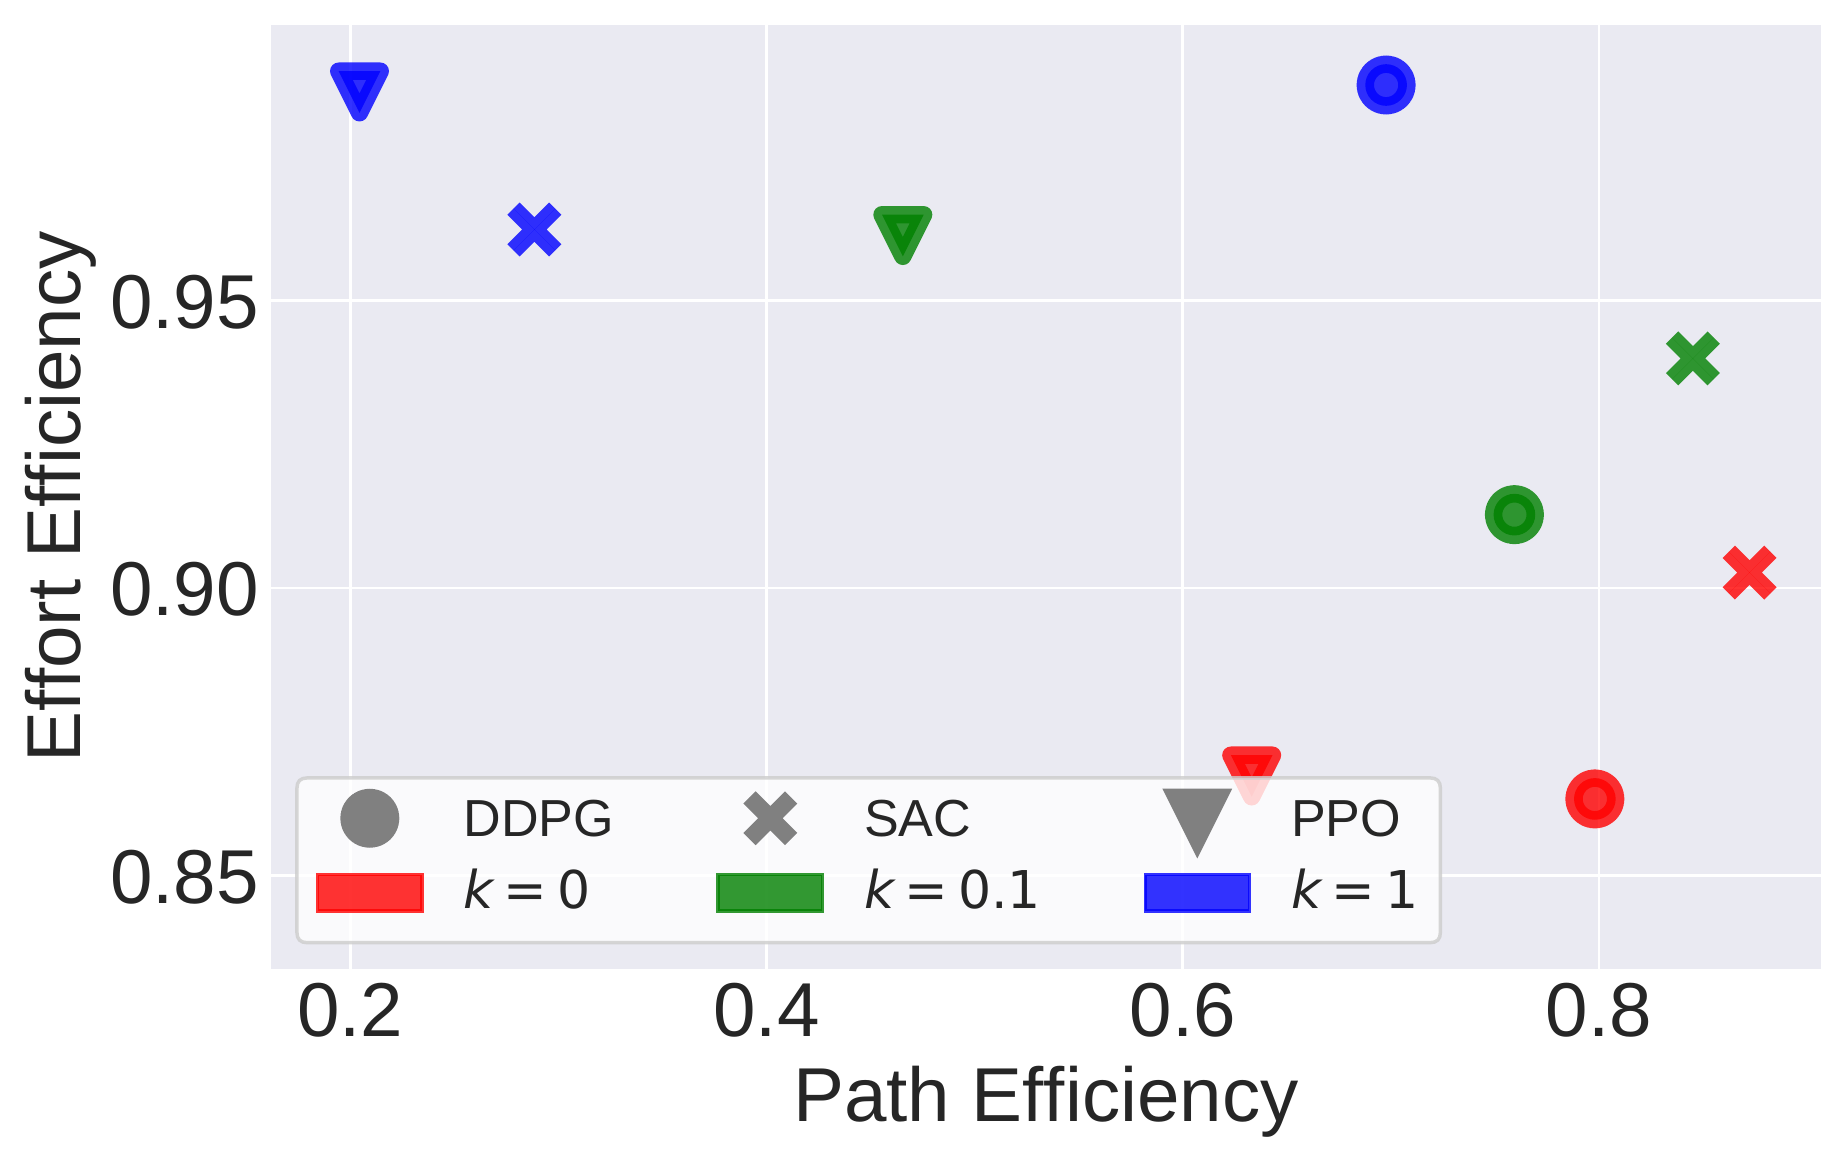}
  \end{center}
  	\caption{\footnotesize \textbf{Trade-off between Path and Effort Efficiency for Turtlebot.} }
	\label{fig:trade_off_turtlebot}
	\vspace{-4mm}
\end{figure}

\begin{figure}[h]
  \begin{center}
    \includegraphics[width=0.96\columnwidth]{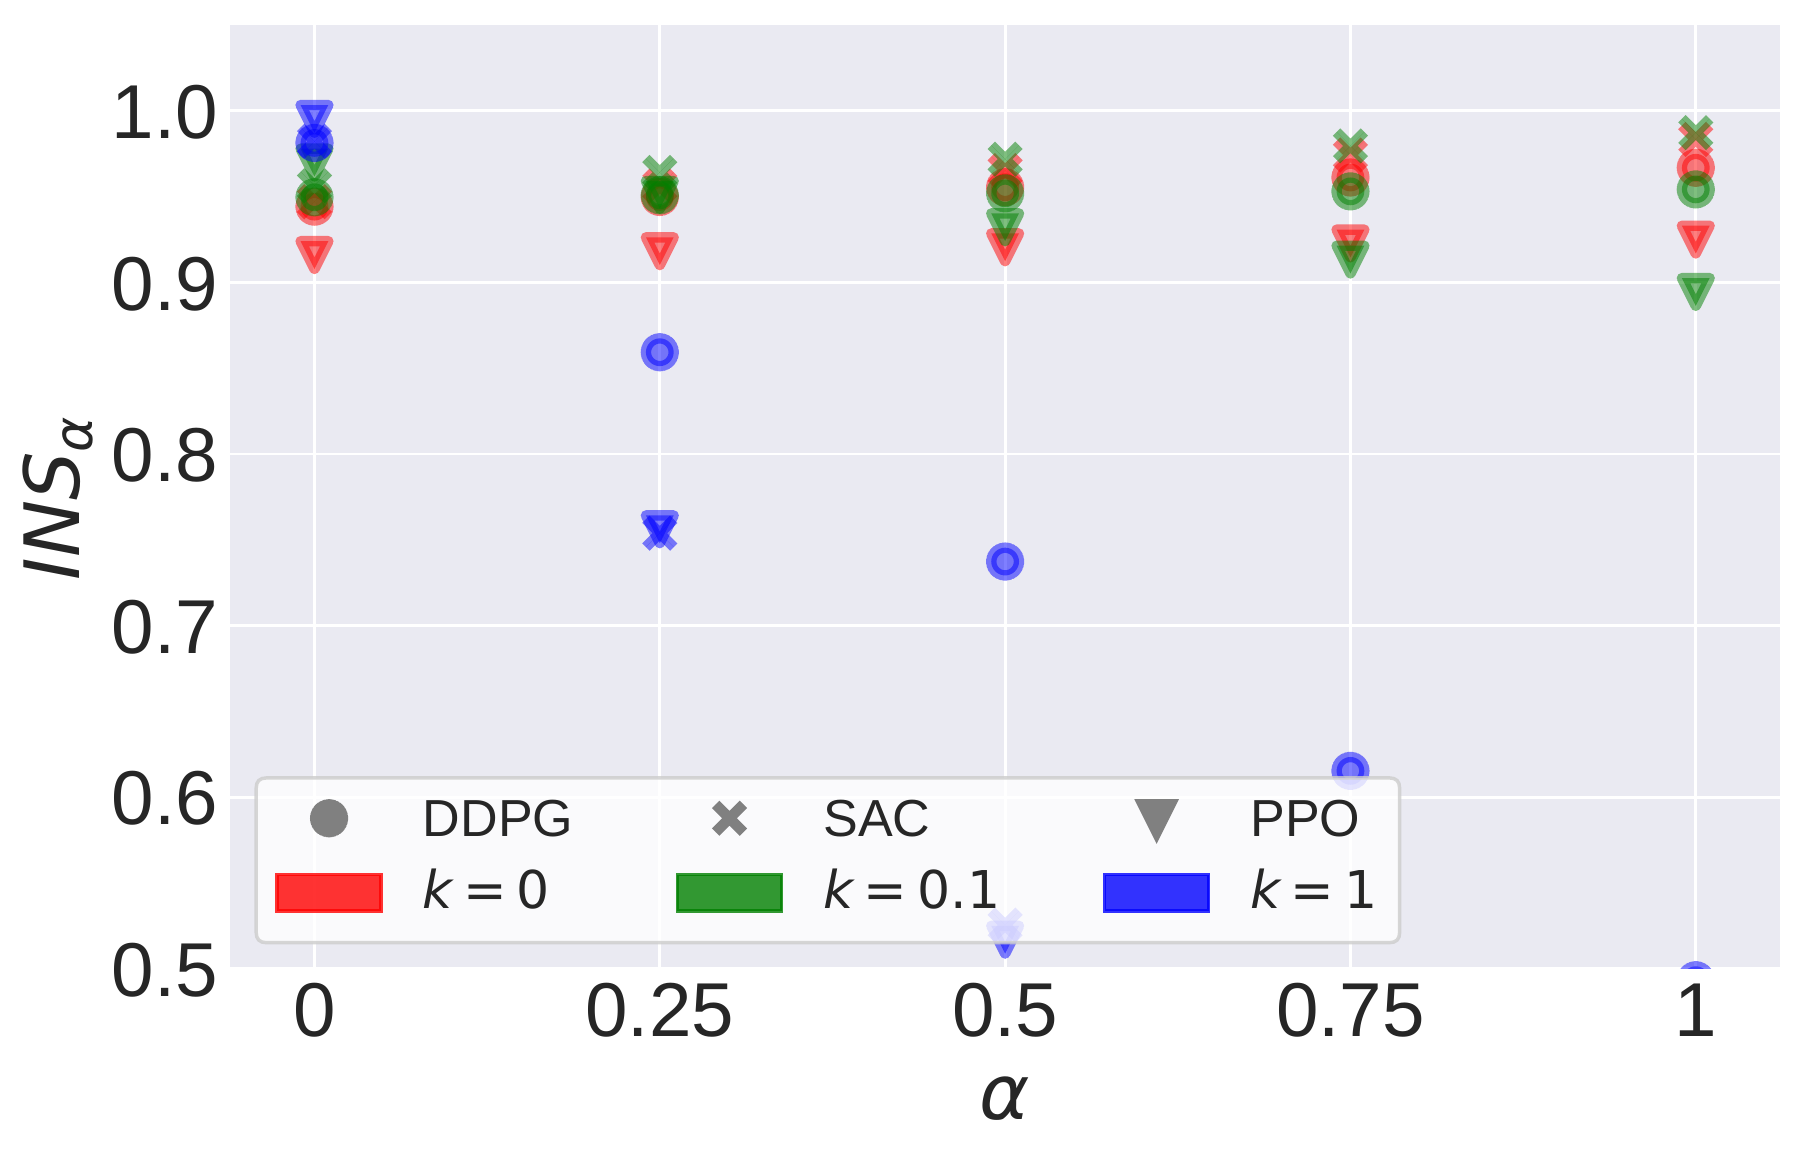}
  \end{center}
	\vspace{-3mm}
  \caption{\footnotesize \textbf{Interactive Navigation Score ($\textrm{INS}$) at different $\alpha$ levels for Fetch.} }
	\label{fig:ins_fetch}		
	\vspace{-4mm}
\end{figure}

Finally, we examined the $INS_{0.5}$ on training set and test set. There is no statistical difference between performance on training set and test set, as can be seen in Fig.~\ref{fig:stat}. 

\begin{figure}[h]
  \begin{center}
    \includegraphics[width=0.96\columnwidth]{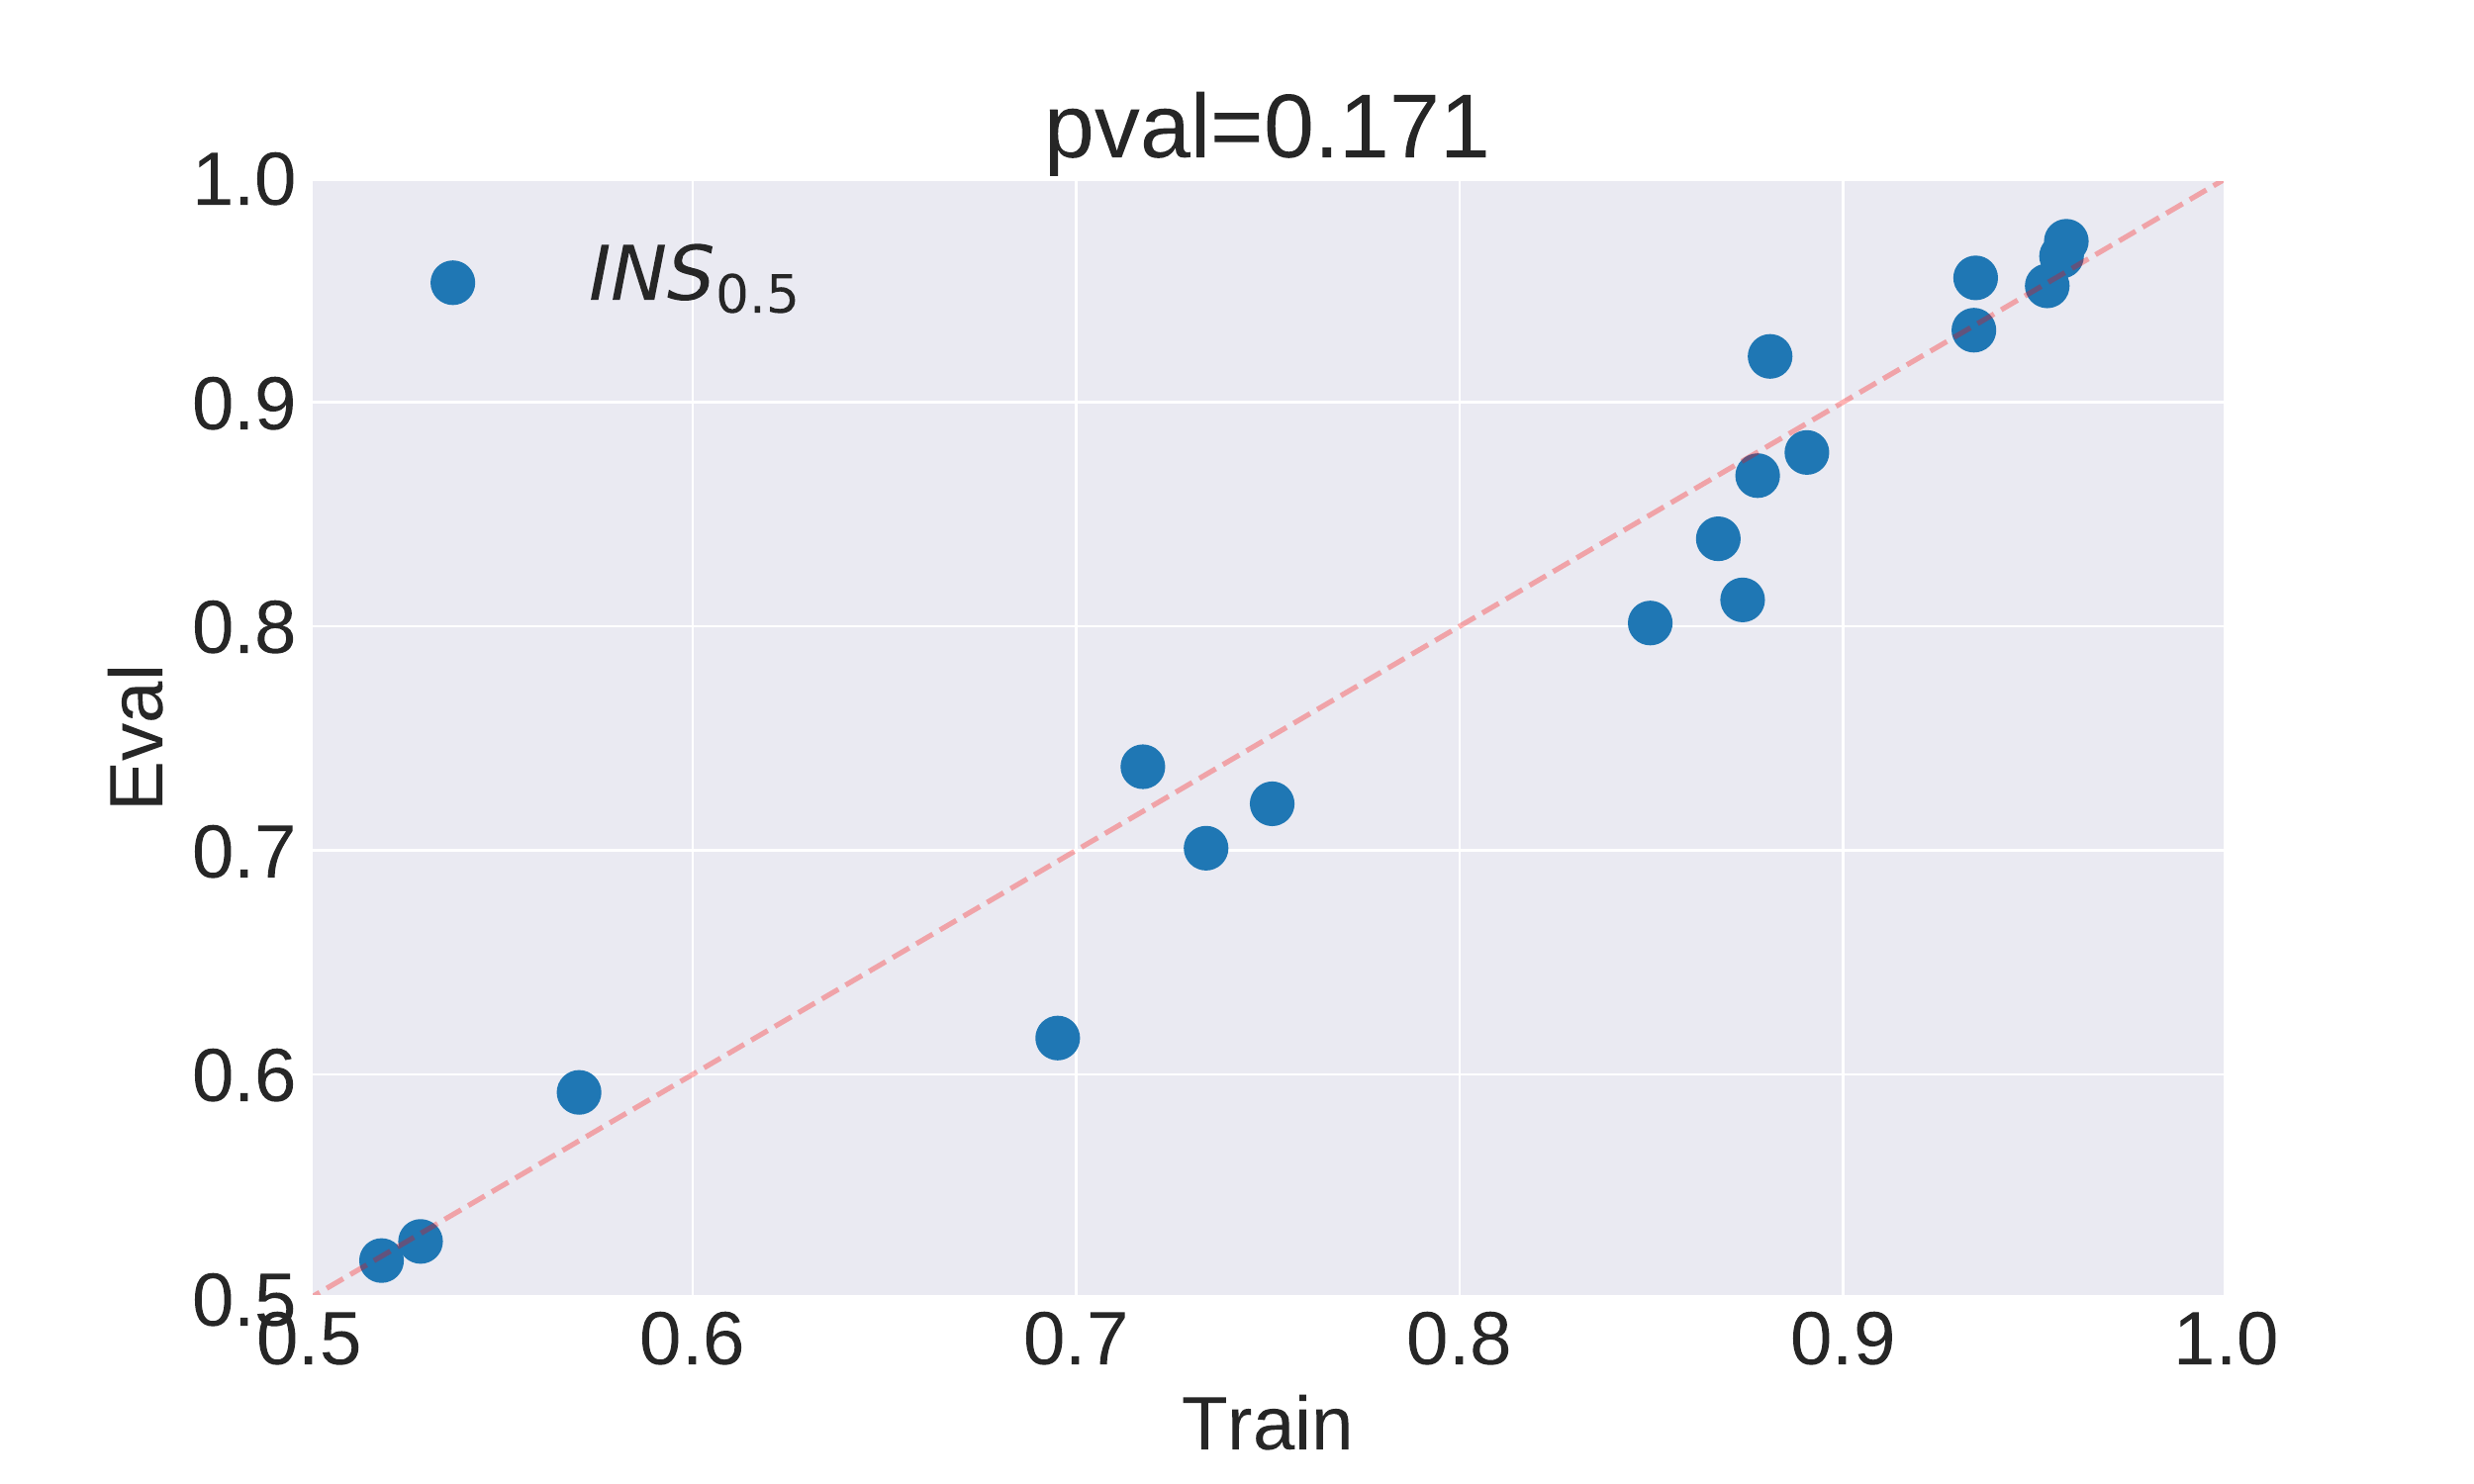}
  \end{center}
  	\caption{Statistical test shows there is no performance drop in terms of INS on test set compared with training set.}
	\label{fig:stat}
	\vspace{-4mm}
\end{figure}
